# Supplementary material for: Estimation of temperature and precipitation uncertainties using quantile neural networks
Source: arXiv:2601.17243 ancillary file (2026-01-24)
Supplement: Supplementary file 1 [file si_template_2019.pdf]

# Supporting Information for “Estimation of temperature and precipitation uncertainties using quantile neural networks”

Andrew Brettin<sup>1</sup> and Laure Zanna<sup>1</sup>

<sup>1</sup>Courant Institute of Mathematical Sciences, New York University, New York, NY, USA

## Contents of this file

1. Figure S1: Pinball function used for optimization in the quantile neural network.
2. Figure S2: Expected quantile loss as a function of quantile probability levels.
3. Figure S3: Timeseries and histograms of samples for Synthetic Dataset 3.
4. Figure S4: Ensemble mean state vector magnitude timeseries for Synthetic Dataset 3.
5. Figure S5 Signed quantile errors on synthetic datasets as a function of the inputs.
6. Figure S6: Histograms of sample mean CRPS for all 1,501 GSOD weather stations.
7. Figure S7: Relationship between quantile neural network skill over the Gaussian maximum likelihood network as a function of the variance explained by the deterministic functional.

---

Corresponding author: A. Brettin, Center for Atmosphere Ocean Science, Courant Institute of Mathematical Sciences, New York University, 251 Mercer St, New York, NY, USA. (brettin@cims.nyu.edu)

8. Table S1: Hyperparameter configurations for different datasets.

9. Table S2: Average number of test samples resulting in quantile crossings for different quantile neural network techniques.

10. Table S3: Proportion of ensemble members which result in no quantile crossings over all samples.

11. Table S4: Hyperparameters varied for training stability analysis.

**Introduction** This document contains additional supporting figures and tables for Brettin and Zanna (2026).

Figure S1 shows the quantile regression loss function for various quantile probability levels  $q$ , while Figure S2 shows the expected quantile loss as a function of  $q$  for different distributions. Figure S3 illustrates the probability distribution for Synthetic Dataset 3 generated by a dynamical process, while Figure S4 demonstrates the ergodicity of the distribution. Figure S5 shows the quantile errors for linear quantile regression, the mean-variance estimation networks, and the RBLQNN as a function of the inputs  $x$ . Figure S6 shows the histograms of sample-mean CRPS for various conditional probability estimation techniques over all 1,501 GSOD weather stations. Figure S7 illustrates the relationship between quantile neural network skill (with respect to the mean-variance estimation network) and the proportion of variance explained by the deterministic functional (MSE network).

Table S1 gives the hyperparameter configurations used on each of the different datasets. Tables S2 and S3 provide metrics for assessing the number of quantile crossings for each of the different quantile neural network methods considered. Table S4 shows the hyperparameters used in a grid search for the training stability analysis in Section 3.3.

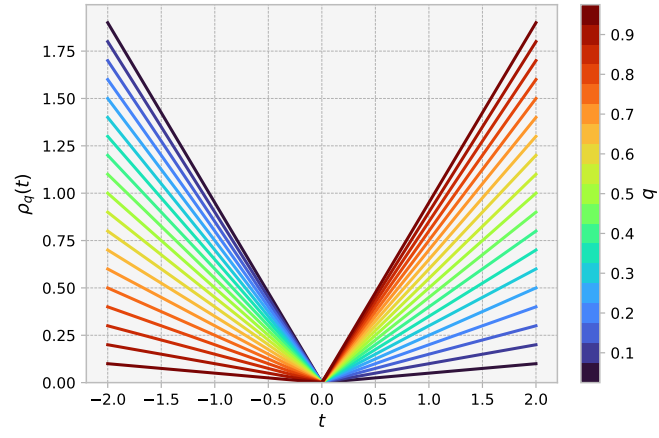

**Figure S1.** Pinball function used as a quantile loss (Eq. 4).

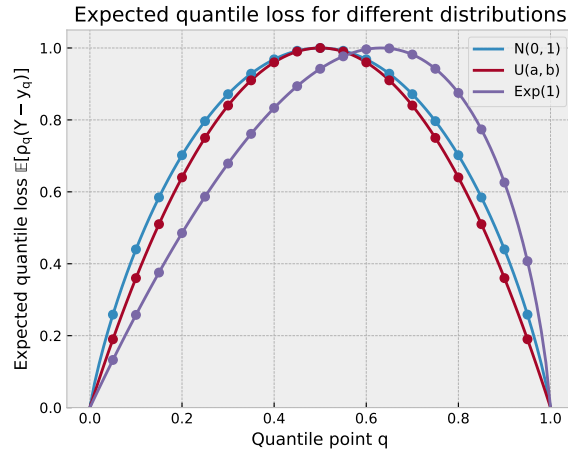

**Figure S2.** Expected quantile loss  $\mathbb{E}[\rho_q(Y - y_q)]$  as a function of quantile probability levels  $q$  for normal (blue), uniform (red), and exponential distributions (purple).

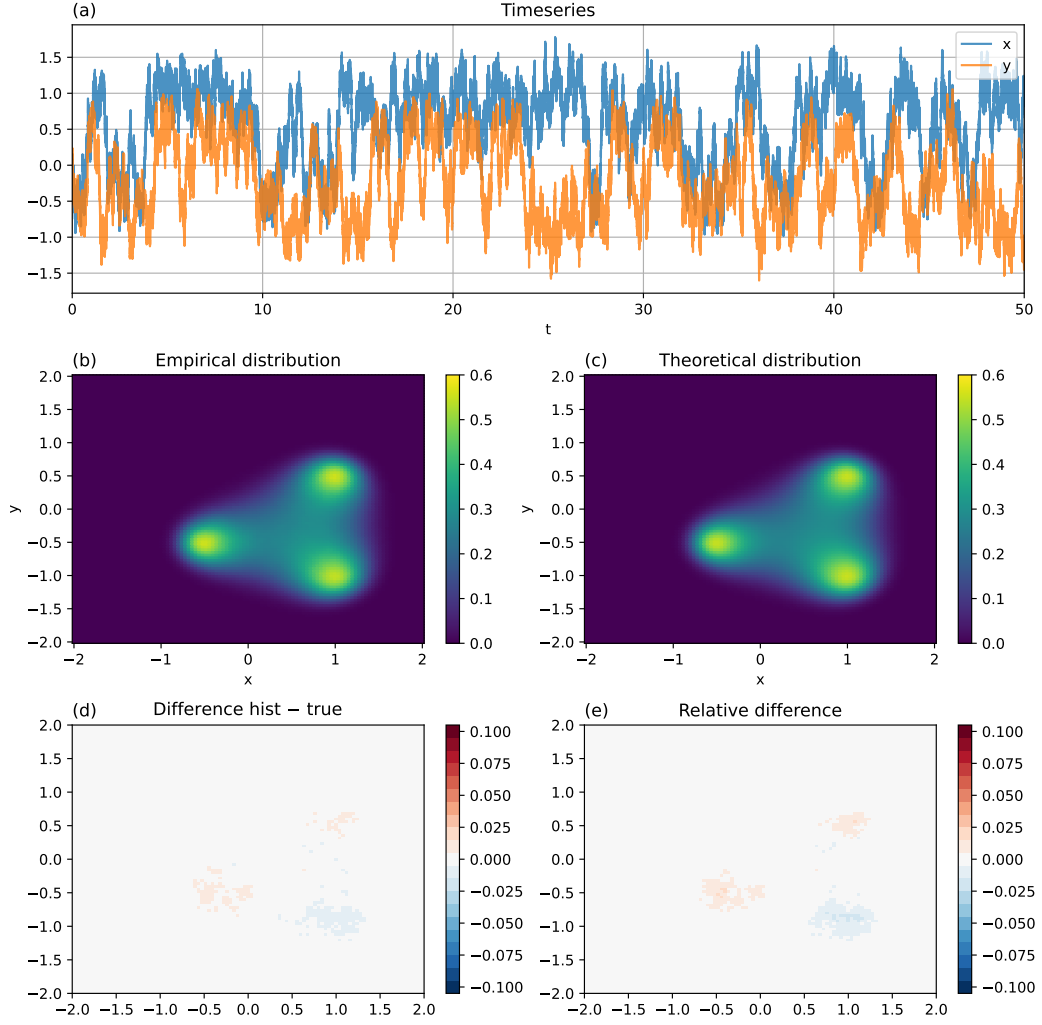

**Figure S3.** Timeseries and histograms of samples generated for Synthetic Dataset 3. (a) Timeseries of  $x$  (blue) and  $y$  (orange) components of the potential system (Eq. 19) for the for times  $0 \leq t \leq 50$ . (b) Joint histogram of samples of  $(x, y)$  for times  $0 \leq t \leq 10,000$ . (c) Theoretical stationary distribution given by the Fokker-Planck equation (the Boltzmann distribution  $e^{-V(x,y)}$ ) for the potential given in Eq. 20. (d) Difference between the empirical histogram (c) and true density (d),  $\tilde{f} - f$ . (e) Relative difference between the histogram and true density  $(\tilde{f} - f)/f$ .

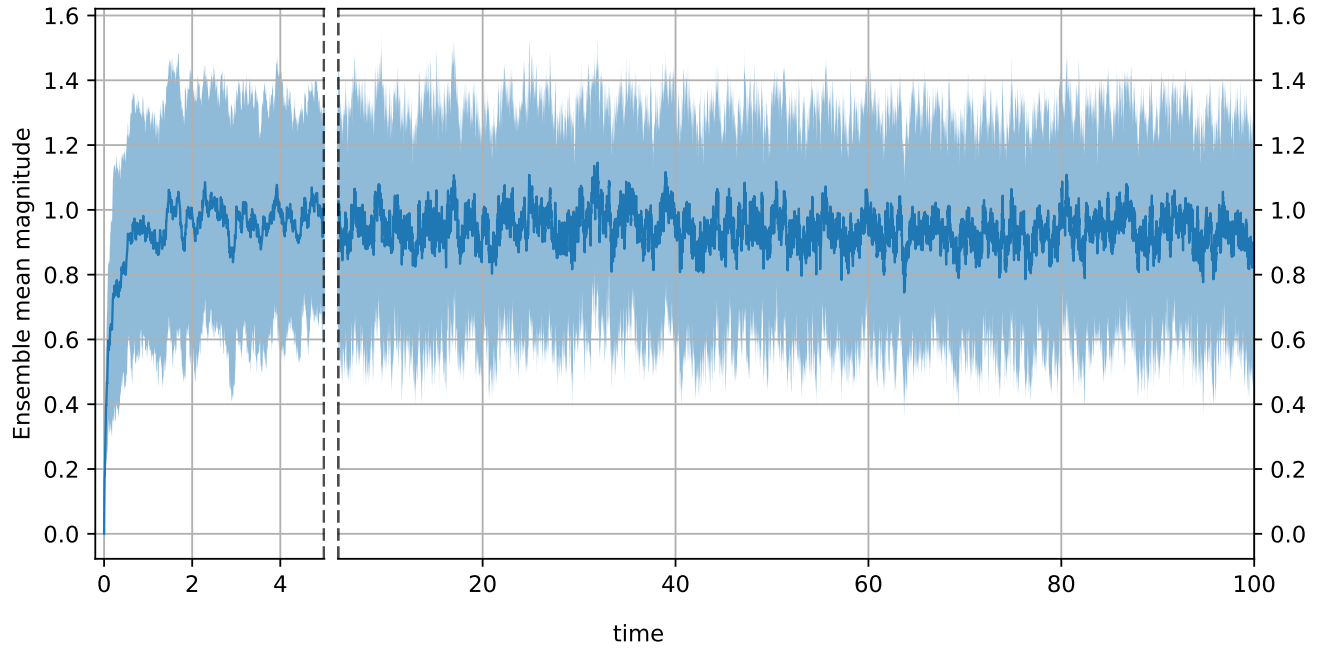

**Figure S4.** Ensemble mean position vector magnitude  $\|(x, y)\|_2$  over 50 different trajectories for the first 100 seconds of simulation time. Shading indicates the ensemble spread ( $\pm 1\sigma$ ).

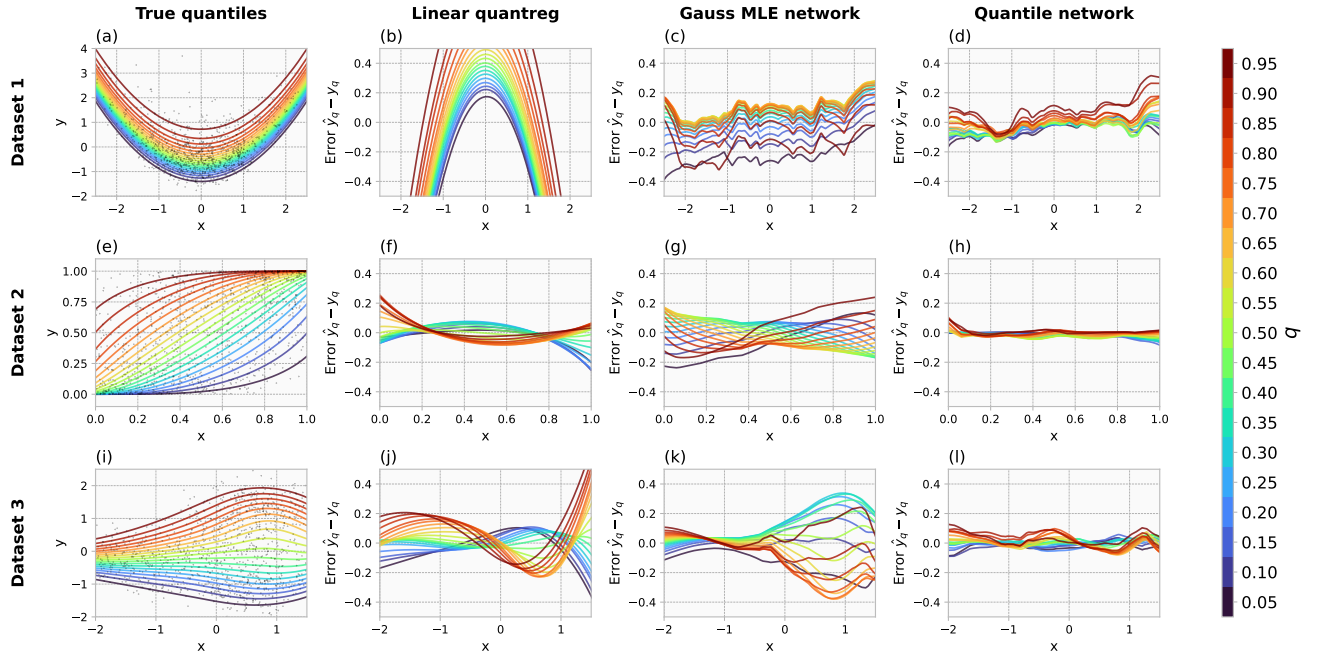

Figure S5. Quantile errors  $\hat{y}_q - y_q$  as a function of  $x$ .



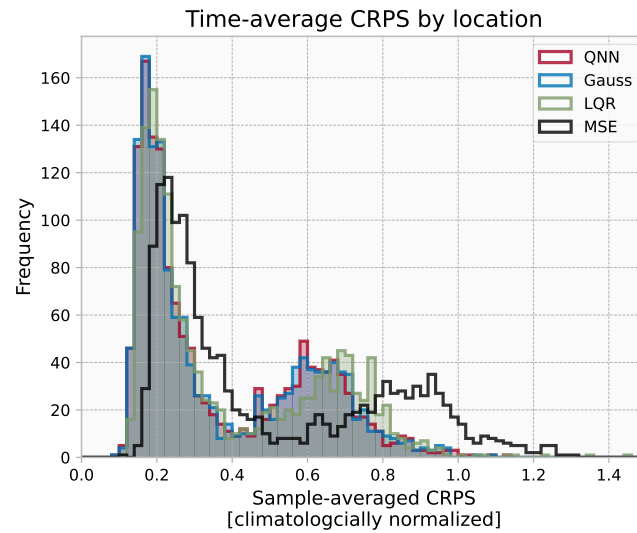

**Figure S6.** Histogram of sample-mean CRPS over all 1,501 GSOD stations for quantile neural network (red), Gaussian maximum likelihood network (blue), linear quantile regression (green), and MSE network (black). Values have been standardized with respect to the climatological CRPS at each location.

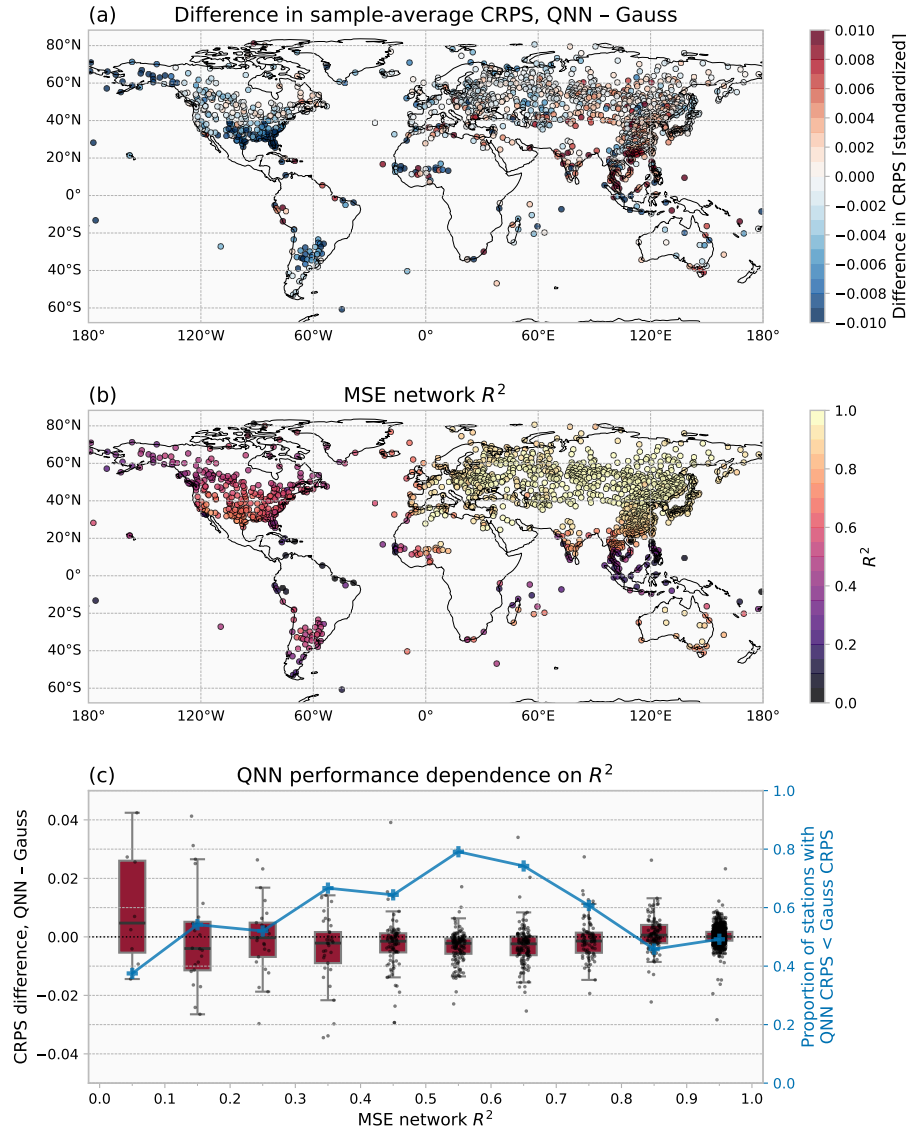

**Figure S7.** Relationship between CRPS gain from Gaussian maximum likelihood network to quantile neural network and coefficient of determination for MSE network. (a) Sample-average CRPS difference between quantile neural network and Gaussian maximum likelihood network, as in Figure 7d. (b) Coefficient of determination ( $R^2$ ) for MSE network. (c) Boxplots of CRPS difference conditioned on corresponding station MSE network  $R^2$  (binned into tenths), with strip plots (black dots) indicating individual stations. Blue line indicates the proportion of stations with lower CRPS for the quantile neural network.

**Table S1.** Hyperparameter configurations for different datasets.

| Hyperparameter                | Synthetic datasets | GSOD dataset | TRMM dataset |
|-------------------------------|--------------------|--------------|--------------|
| Hidden layers                 | 3                  | 3            | 3            |
| Neurons per hidden layer      | 128                | 128          | 100          |
| Bias loss weight $\eta$ (QNN) | 1.0                | 0.01         | 0.01         |
| Batch size                    | 256                | 256          | 256          |
| Optimizer                     | Adam               | Adam         | Adam         |
| Learning rate <sup>†</sup>    | $10^{-3}$          | $10^{-5}$    | $10^{-5}$    |
| $L_2$ regularization          | $10^{-5}$          | $10^{-2}$    | $10^{-2}$    |
| Maximum epochs                | 1,000              | 1,000        | 1,000        |
| Early stopping epochs         | 25                 | 300          | None         |
| Warmup epochs                 | 100                | 100          | 100          |
| Prescribed variance           | 0.1                | 0.1          | 0.1          |

<sup>†</sup> For the linear quantile regression model, a larger learning rate of  $10^{-3}$  is used to expedite convergence for the 1,501 stations in the GSOD dataset; this improved validation performance and was justified by the convexity of the optimization problem.

**Table S2.** Number of test samples (out of 1,000) resulting in quantile crossings for each quantile neural network technique, averaged over all 100 ensemble members.

| Dataset | Quantile NN | Unweighted | No bias | Cumulative inc. |
|---------|-------------|------------|---------|-----------------|
| 1       | 2.1         | 6.06       | 5.5     | 0.0             |
| 2       | 26.5        | 266.2      | 258.8   | 0.0             |
| 3       | 0.0         | 0.50       | 1.1     | 0.0             |

**Table S3.** Proportion of ensemble members resulting in no quantile crossings over all samples.

| Dataset | Quantile NN | Unweighted | No bias | Cumulative inc. |
|---------|-------------|------------|---------|-----------------|
| 1       | 0.38        | 0.02       | 0.05    | 1.0             |
| 2       | 0.48        | 0.00       | 0.00    | 1.0             |
| 3       | 0.98        | 0.79       | 0.76    | 1.0             |

**Table S4.** Hyperparameters used for training stability analysis.

| Hyperparameter     | Values considered |           |           |           |           |           |           |           |
|--------------------|-------------------|-----------|-----------|-----------|-----------|-----------|-----------|-----------|
| Learning rate      | $10^{-8}$         | $10^{-7}$ | $10^{-6}$ | $10^{-5}$ | $10^{-4}$ | $10^{-3}$ | $10^{-2}$ | $10^{-1}$ |
| $L_2$ weight decay | 0                 | $10^{-5}$ | $10^{-3}$ |           |           |           |           |           |
| Number of layers   | 2                 | 3         |           |           |           |           |           |           |
| Neurons per layer  | 64                | 128       | 256       |           |           |           |           |           |
